# Supplementary material for: Diffusion Dynamics and Optimal Coupling in Directed Multiplex Networks
Source: arXiv:1708.01951 source file (2017-08-07)
Supplement: Supplementary file 1 [file MultiplexDirectedNetworksv_SM.pdf]

# Supplemental Material

## Diffusion Dynamics and Optimal Coupling in Directed Multiplex Networks

Alejandro Tejedor[1], Anthony Longjas[1], Efi Foufoula-Georgiou[1], Tryphon Georgiou[2], and Yamir Moreno[3,4,5]

[1]Department of Civil and Environmental Engineering, University of California, Irvine, Irvine, CA 92697, USA
[2]Department of Mechanical and Aerospace Engineering, University of California, Irvine, Irvine, CA 92697, USA
[3]Institute for Biocomputation and Physics of Complex Systems (BIFI), Universidad de Zaragoza, 50018 Zaragoza, Spain
[4]Departamento de Física Teórica, Universidad de Zaragoza, 50009 Zaragoza, Spain
[5]Institute for Scientific Interchange, ISI Foundation, Turin, Italy

## Mekong Delta

**Mekong Delta:** The Mekong delta is located in Southern Vietnam (10.1°, 150.6°) and receives input from the Mekong River with an average water discharge of 14 770 $m^3s^{-1}$ and sediment discharge of 1.60 x $10^7$ tons $yr^{-1}$ [*Syvitski et al.*, 2005]. In terms of land area (~50,000 $km^2$), it is the third largest delta on Earth, and with nearly 20 million people, it is one of the most densely populated regions in the world [*General Statistics Office*, 2012]. The delta with its agricultural and aquaculture industries is one of the most important sources of food supply in Asia [*WWF*, 2012]. However, floods, coastal erosion, salt water intrusion and hydrologic changes due to hydropower projects in the upstream of the Mekong are threatening the state of this critical region and its inhabitants.

**Delta channel network.** We represent the delta channel network as a graph, where the edges represent channels, and nodes correspond to the locations where one channel splits into new channels (bifurcation) or two or more channels merge into a single channel (confluence) (see Fig. 3 – left panel). All the channels that connect the apex (inlet) of the delta to the shoreline, with widths equal or larger than 50 m, are considered in this network. The network consists of 253 nodes and 374 links.

**Mekong Delta multiplex.** We define a two-layer multiplex based on the channel network of the Mekong delta. Layer 1 consists of the directed channel network, where the direction of the edges corresponds to the main direction of water flow; and Layer 2 consists of the undirected counterpart of the network in Layer 1. Note that the outlet nodes (nodes located at the shoreline that drain water directly to the ocean) of the delta have been reconnected to the apex (inlet) by

adding edges to guarantee that the directed layer consists of a strongly connected network. Furthermore, *Tejedor et al.* [2015] showed that by using the cycled version of the network (i.e., containing the additional edges that connect the outlets of the system to its inlet) argued there as a constraint to acknowledge conservation of mass, the steady state distribution of fluxes can be computed as the eigenvector corresponding to the zero eigenvalue of the directed Laplacian of the network.

## Figures

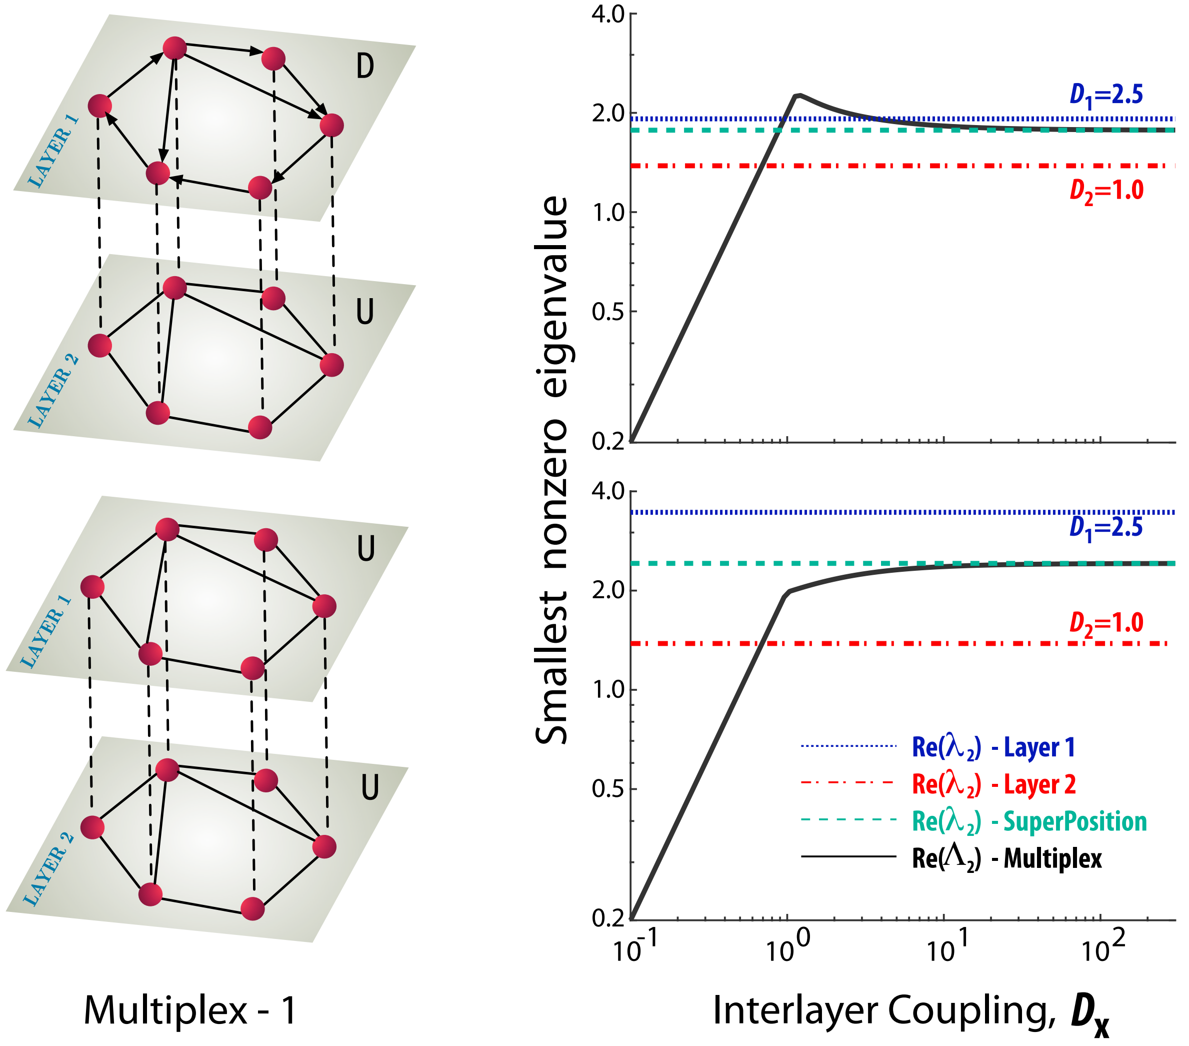


**FIG S1. Characteristic rate of convergence to stationary state solution of a Continuous Time Markov Chain on Multiplex-1 and its undirected counterpart.**

*(Top panel) Directed Multiplex-1* consists of a directed network (layer 1) and its undirected counterpart (layer 2) – this example serves to illustrate the effect of directionality in only one of the layers. We compare the characteristic time of convergence to steady state of a diffusion-like process acting on this multiplex with that of its undirected counterpart (Und*irected Multiplex-1 -*

bottom panels). Fig. S1 (right panels) shows the value of the smallest (in terms of its real part) nonzero eigenvalue $\mathrm{Re}(\Lambda_2)$ of the supra-Laplacian as a function of the interlayer coupling, $D_x$ for both the directed (top) and undirected multiplex, and for the same pair of diffusion coefficients $(D_1, D_2) = (2.5, 1.0)$. We highlight the existence of an optimal coupling that is only exhibited by the directed multiplex ($D_x \sim 1.2$) wherein the rate of convergence to the steady state is the fastest (even faster than for fully coupled layers – the asymptotic limit, green line).

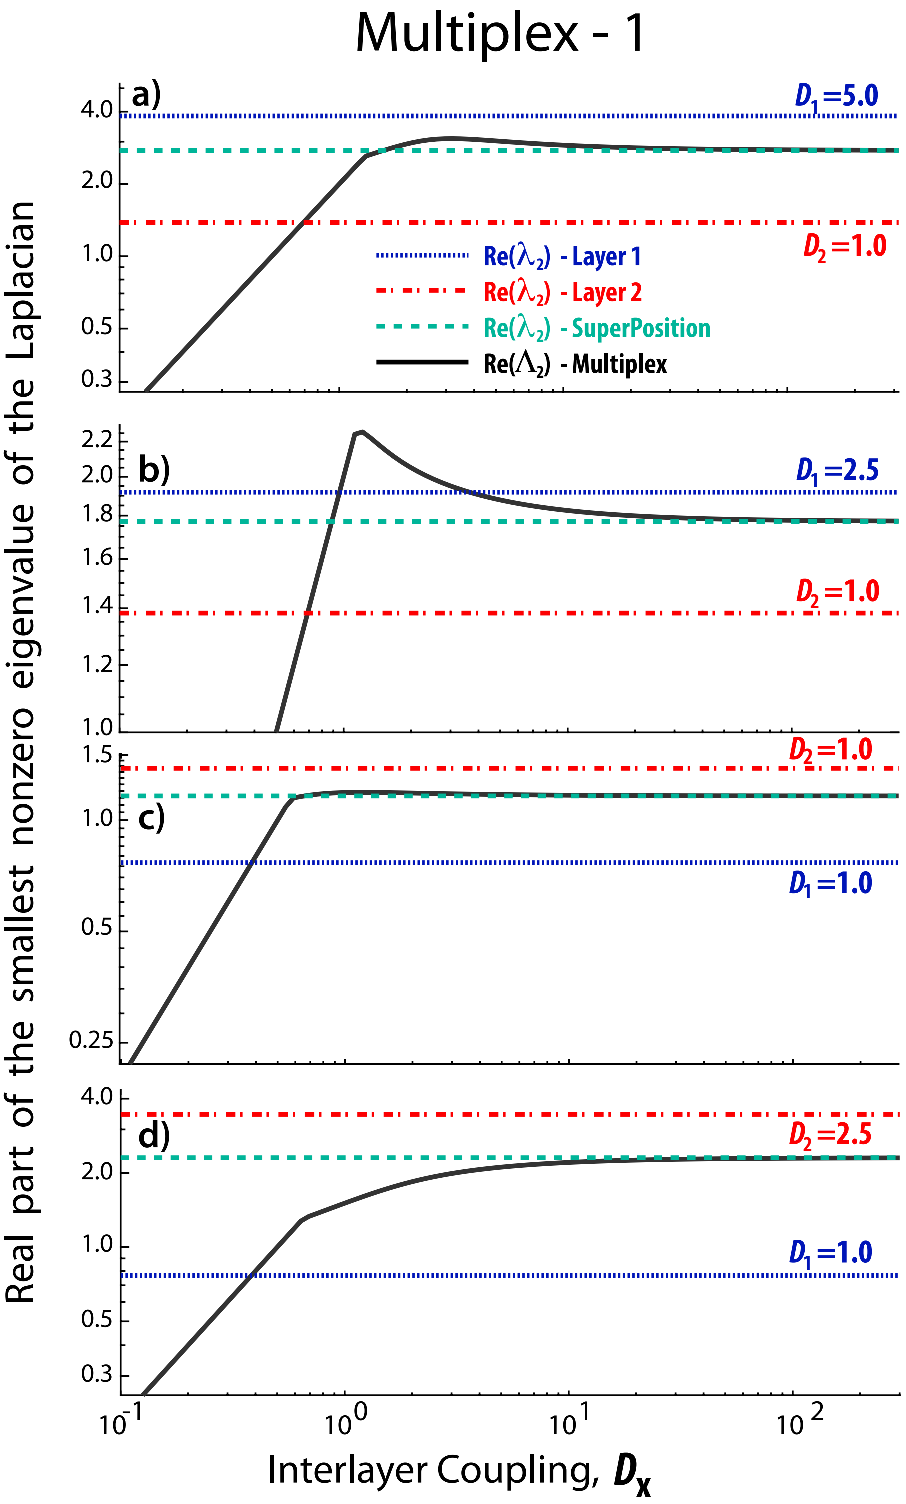


**FIG S2. Characteristic rate of convergence to stationary state solution of a Continuous Time Markov Chain on Multiplex-1 for different pairs ($D_1, D_2$).**

Fig. S2 shows the value of the smallest (in terms of its real part) nonzero eigenvalue $\mathrm{Re}(\Lambda_2)$ of the supra-Laplacian as a function of interlayer coupling, $D_x$. From this figure we highlight the following important observations: (**i**) We first observe that for pairs of $D_1$ and $D_2$ where the rate of convergence to steady state is larger for the directed layer ($\mathrm{Re}(\lambda_2^1)$, superscript 1 refers to layer 1 – blue line) than for the undirected network ($\mathrm{Re}(\lambda_2^2)$ superscript 2 refers to layer 2 – red line) an optimal coupling emerges where the maximum $\mathrm{Re}(\Lambda_2)$ for the multiplex network (black line) is achieved exhibiting higher values than those observed for the asymptotic limit (green line) (see panels a and b). (**ii**) In panel b ($D_1$=2.5 $D_2$=1.0), the rates of convergence to steady state in the individual layers $\mathrm{Re}(\lambda_2^1)$ and $\mathrm{Re}(\lambda_2^2)$ are very similar, and therefore each individual layer has similar transport properties. This multiplex configuration, when working at optimal coupling regime, is characterized by much faster rates of convergence to the stationary solution than the rates of the individual layers, exhibiting a superdiffusive behavior (even though no superdiffusive behavior is observed in the asymptotic limit). (**iii**) Panel c ($D_1$=$D_2$=1) illustrates a scenario in which although the directed network is slightly slower than the undirected network $\mathrm{Re}(\lambda_2^1) \lesssim \mathrm{Re}(\lambda_2^2)$ for intermediate values of coupling, $\mathrm{Re}(\Lambda_2)$ can exceed the asymptotic values for $D_x \to \infty$. (**iv**) Finally, panel d shows a scenario where the undirected layer is substantially faster than the directed layer ($\mathrm{Re}(\lambda_2^2) > \mathrm{Re}(\lambda_2^1)$ ). This multiplex network, although directed, when subject to a diffusion process, present dynamics dominated by its undirected (faster) layer. Consequently, the trends observed in panel d, especially the lack of an optimal coupling regime, are comparable with those reported for undirected multiplex networks [e.g., *Gomez et al*., 2013].

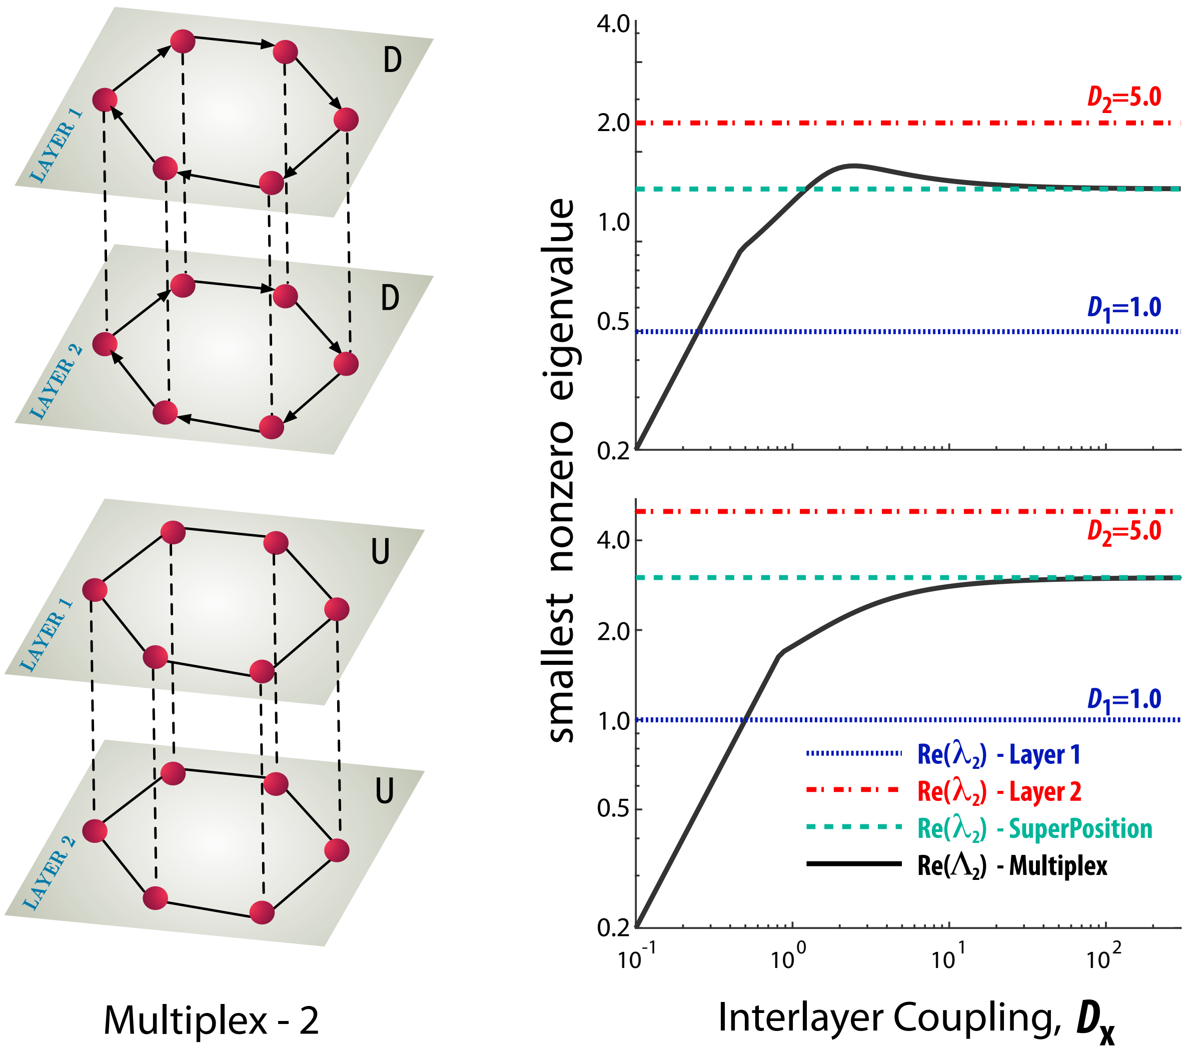


**FIG S3. Characteristic rate of convergence to stationary state solution of a Continuous Time Markov Chain on Multiplex-2 and its undirected counterpart.**

*(Top panel) Directed Multiplex-2* is composed of the same directed network in the two layers – this example is to illustrate the effect of different rates ($D_1$ vs $D_2$) at the different layers. We compare the characteristic time of convergence to steady state of a diffusion-like process acting on this multiplex with that of its undirected counterpart (Und*irected Multiplex-2* - bottom panels). Fig. S3 (right panels) shows the value of the smallest (in terms of its real part) nonzero eigenvalue Re($\Lambda_2$) of the supra-Laplacian as a function of interlayer coupling, $D_x$ for both the directed (top) and undirected multiplex, and for the same pair of diffusion coefficients ($D_1$, $D_2$) =

(1.0, 5.0). We highlight the existence of an optimal coupling that it is only exhibited by the directed multiplex ($D_x$~2.4) , wherein the rate of convergence to the steady state is the fastest (even faster than for fully couple layers - asymptotic limit, green line).

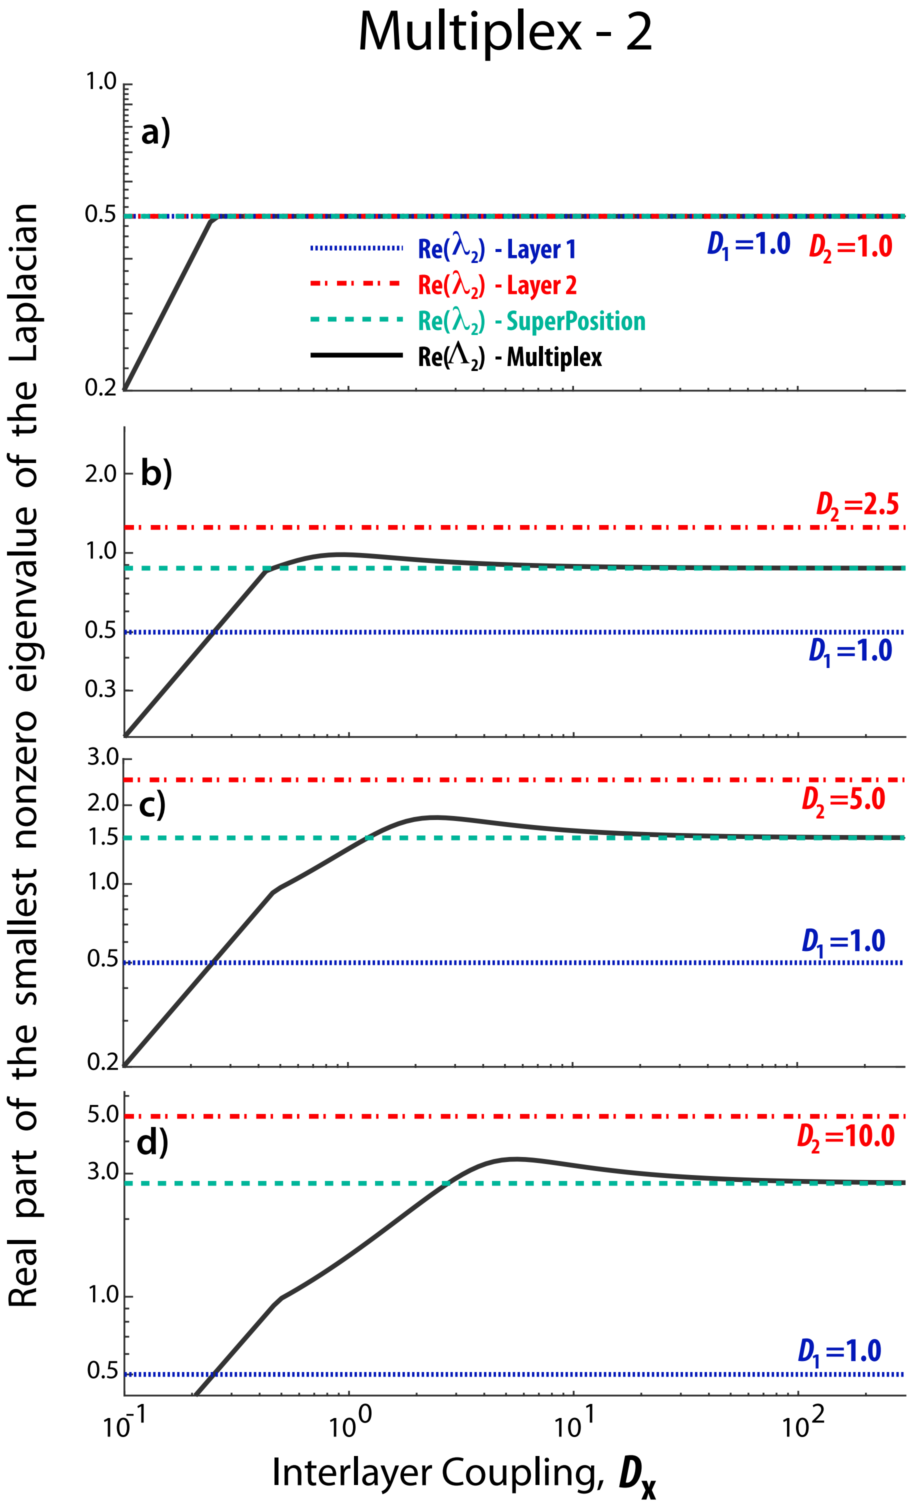


**FIG S4. Characteristic rate of convergence to stationary state solution of a Continuous Time Markov Chain in Multiplex-2 for different pairs ($D_1$, $D_2$).**

Fig. S4 shows the value of the smallest (in terms of its real part) nonzero eigenvalue $\mathrm{Re}(\Lambda_2)$ of the supra-Laplacian as a function of interlayer coupling, $D_x$. From Fig. S4 we highlight the following important observations: (**i**) We first report in panel a, the trivial case ($D_1$=$D_2$=1), for which both the topologies and the diffusion coefficients are identical in both layers. The multiplex network, as expected, converges asymptotically with a rate identical to its individual layers. (**ii**) Panels b, c and d show a similar emerging behavior: when the diffusion coefficients of the two layers differ, an optimal coupling exists where the rate of convergence is the fastest. There are two main phenomena that when combined give rise to the emergence of this optimum transport regime: (1) the different diffusion coefficients in the different layers form distinct dynamical paths (meaning same topological paths but with different speeds) that enhance the mixing. (2) For intermediate values of coupling, the two layers contribute substantially to the total transport (the random walker spends time in both layers) but keeping a certain degree of independence in their dynamics, in contrast with high coupling scenarios (where the transport across counterpart nodes in different layers is fastest, acting as a constraint in the dynamics of all the layers, since similar gradients of concentration will appear among different nodes within each of the layers).

Note that in this case we do not present results for values of $D_1$ exceeding $D_2$ for an obvious symmetry in the dynamics of the multiplex since the two layers are identical.

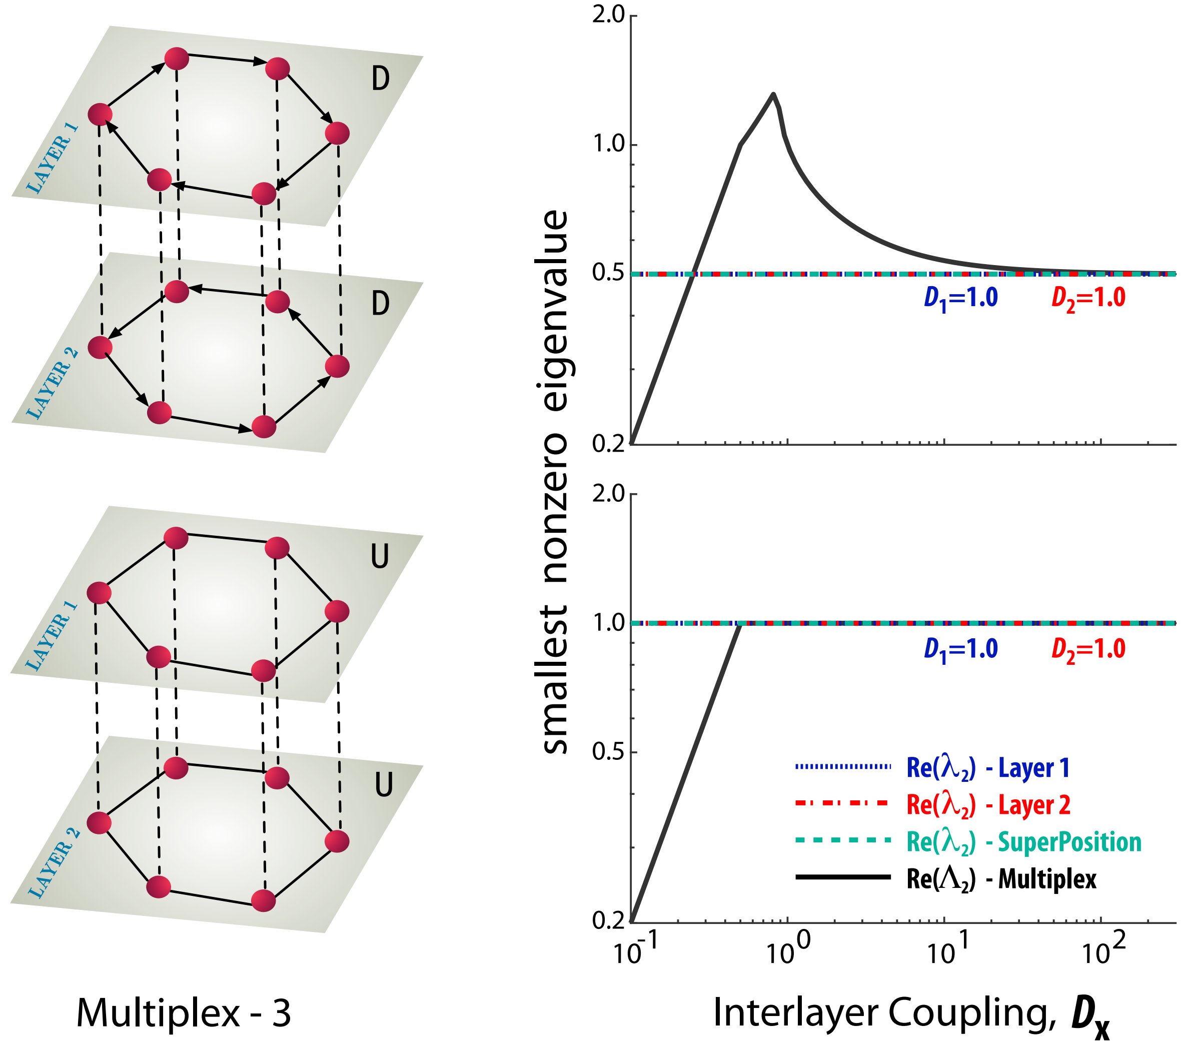


**FIG S5. Characteristic rate of convergence to stationary state solution of a Continuous Time Markov Chain on Multiplex-3 and its undirected counterpart.**

*(Top panel) Directed Multiplex-3* where the network present in layer 1 is the reverse (opposite directionality of all the edges) of the network in layer 2 – this example serves to illustrate the effect of directionality when the topology and rates of transition are the same. We compare the characteristic time of convergence to steady state of a diffusion-like process acting on this multiplex with that of its undirected counterpart (Und*irected Multiplex-3* - bottom panels). Fig. S5 (right panels) shows the value of the smallest (in terms of its real part) nonzero eigenvalue Re($\Lambda_2$) of the supra-Laplacian as a function of interlayer coupling, $D_x$ for both the directed (top)

and undirected multiplex, and for the same pair of diffusion coefficients ($D_1$, $D_2$) = (1.0, 1.0). We highlight the existence of an optimal coupling that it is only exhibited by the directed multiplex ($D_x \sim 0.8$), wherein the rate of convergence to the steady state is the fastest (even faster than for fully couple layers - asymptotic limit, green line). Furthermore, in this example the rate of convergence observed in the directed multiplex at the optimal coupling is even faster than the fastest rate computed for its undirected counterpart.

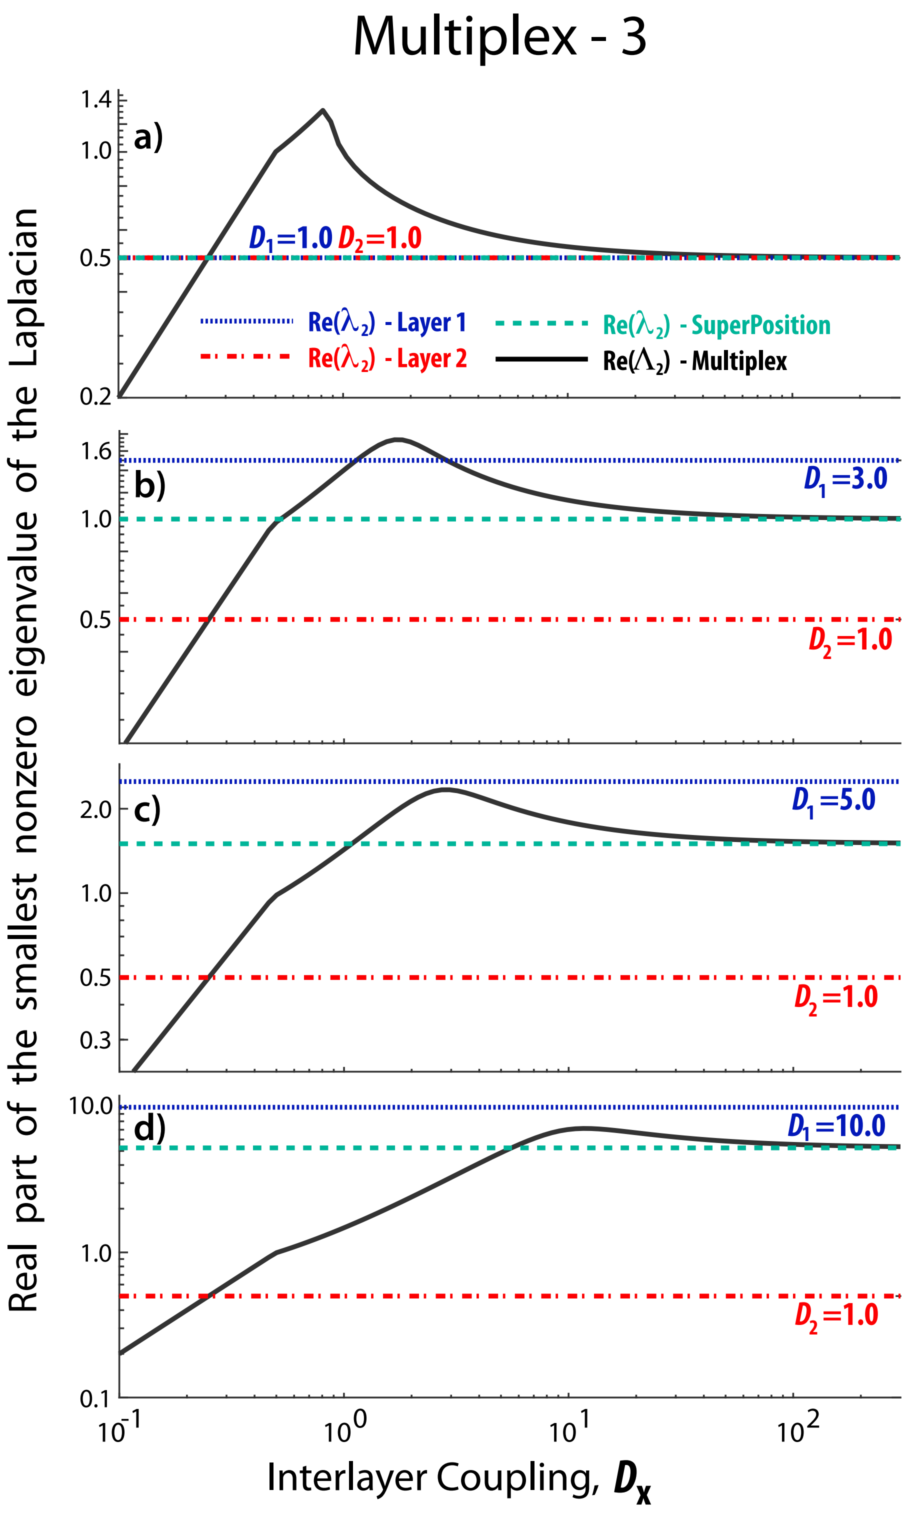


**FIG S6. Characteristic rate of convergence to stationary state solution of a Continuous Time Markov Chain in Multiplex 3 for different pairs ($D_1, D_2$).**

Fig. S6 shows the value of the smallest (in terms of its real part) nonzero eigenvalue $\mathrm{Re}(\Lambda_2)$ of the supra-Laplacian as a function of interlayer coupling, $D_x$. From Fig. S6 we highlight the following important observations: (**i**) The exploration of different values of the intralayer diffusion coefficients (panels a-d) show the existence of an optimal coupling for intermediate values of $D_x$ where the rate of convergence of the multiplex network is the fastest. There are two main phenomena that when combined give rise to the emergence of this optimum transport regime: (1) the different directionality of the paths in the different layers enhances the mixing. This phenomenon requires a high enough value of coupling to make the alternative paths in different layers accessible (i.e., the probability of transition between layers has to be significant). (2) For intermediate values of coupling, the two layers contribute substantially to the total transport (the random walker spends time in both layers) but keeping a certain degree of independence in their dynamics, in contrast with high coupling scenarios (where the transport across counterpart nodes in different layers is fastest, acting as a constraint in the dynamics of all the layers since similar gradients of concentration will appear among different nodes within each of the layers). (**ii**) Precisely when the rate of convergence of the individual layers are similar ($\mathrm{Re}(\lambda_2^1) \sim \mathrm{Re}(\lambda_2^2)$), the rate of convergence in the multiplex is enhanced with respect to the rates of the individual layers. In these scenarios, the overall system presents superdiffusion-like behavior for the optimal coupling regime (e.g., panels a and b), i.e., the rates of convergence that characterize the multiplex are even faster than both of the individual layers.

Note that in this case we do not present results for values of $D_1$ exceeding $D_2$ for obvious symmetry in the dynamics of the multiplex since the two layers are topological identical (one layer is the reverse of the other).

**References:**

General Statistics Office: Statistical Yearbook of Vietnam 2011. Statistical Publishing House, Hanoi (2012).

J. Syvitski, A. Kettner, A. Correggiari, and B. Nelson, Distributary channels and their impact on sediment dispersal, Mar. Geol. **222–223**, 75–94 (2005).

A. Tejedor, A. Longjas, I. Zaliapin, and E. Foufoula-Georgiou, Delta channel networks: 1. A graph-theoretic approach for studying connectivity and steady state transport on deltaic surfaces, Water Resour. Res. **51**, 3998-4018 (2015).

World Wildlife Fund for Nature, Ecological Footprint and Investment in Natural Capital in Asia and the Pacific, World Wildlife Fund, Gland, Switzerland, 103 p. (2012).
